# Supplementary material for: SGPMIL: Sparse Gaussian Process Multiple Instance Learning
Source: arXiv:2507.08711 source file (2026-01-17)
Supplement: Supplementary file 1 [file slide_results_supplementary.tex]

\begin{table*}[ht]
    \centering
    \begin{tabular}{l@{\hskip 2pt}c@{\hskip 2pt}c@{\hskip 2pt}c@{\hskip 2pt}c@{\hskip 2pt}c@{\hskip 2pt}c@{\hskip 2pt}c@{\hskip 2pt}c@{\hskip 2pt}c@{\hskip 3pt}c@{\hskip 2pt}c@{\hskip 2pt}c@{\hskip 2pt}c@{\hskip 2pt}c@{\hskip 2pt}c@{\hskip 2pt}c@{\hskip 2pt}c}
    \midrule
    & \multicolumn{12}{c}{Bag-level}  & \multicolumn{4}{c}{Instance-level} \\    
    \cmidrule(lr){2-13} \cmidrule(lr){14-17}
    \multirow{2}{*}{} 
        & \multicolumn{3}{c}{\textbf{CAMELYON16}} 
        & \multicolumn{3}{c}{\textbf{TCGA-NSCLC}}
        & \multicolumn{3}{c}{\textbf{PANDA}}
        & \multicolumn{3}{c}{\textbf{BRACS}}
        & \multicolumn{4}{c}{\textbf{CAMELYON16}} \\
    \cmidrule(lr){2-4} \cmidrule(lr){5-7} \cmidrule(lr){8-10} \cmidrule(lr){11-13} \cmidrule(lr){14-17}
    & ACC & AUC & ACE
    & ACC & AUC & ACE 
    & ACC & $\kappa$ & ACE
    & ACC & AUC & ACE
    & ACC & F1 & FROC & AUC\\
    \midrule
    \makecell[l]{ABMIL}
        % CAMELYON16
        & \makecell{$.964$ \\ \scriptsize $.010$}
        & \makecell{$\mathbf{.990}$ \\ \scriptsize $.005$}
        & \makecell{$.032$ \\ \scriptsize $.011$}
        % NSCLC
        & \makecell{$.953$ \\ \scriptsize $.003$}
        & \makecell{$.973$ \\ \scriptsize $.009$}
        & \makecell{$.039$ \\ \scriptsize $.008$}
        % PANDA
        & \makecell{$.834$ \\ \scriptsize $.064$}
        & \makecell{$.910$ \\ \scriptsize $.028$}
        & \makecell{$.044$ \\ \scriptsize $.015$}
        % BRACS
        & \makecell{$.694$ \\ \scriptsize $.010$}
        & \makecell{$\underline{.852}$ \\ \scriptsize $.025$}
        & \makecell{$.175$ \\ \scriptsize $.007$}
        % CAMELYON16-PATCH
        & $.752$ & $.481$ & $.736$ & $.883$ \\
    \makecell[l]{CLAM}
        % CAMELYON16
        & \makecell{$\underline{.978}$ \\ \scriptsize $.007$}
        & \makecell{\underline{$.986$} \\ \scriptsize $.007$}
        & \makecell{\underline{$.021$} \\ \scriptsize $.007$}
        % NSCLC
        & \makecell{$.934$ \\ \scriptsize $.014$}
        & \makecell{$.953$ \\ \scriptsize $.004$}
        & \makecell{$.056$ \\ \scriptsize $.016$}
        % PANDA
        & \makecell{$\underline{.867}$ \\ \scriptsize $.061$}
        & \makecell{$.927$ \\ \scriptsize $.025$}
        & \makecell{$.031$ \\ \scriptsize $.018$}
        % BRACS
        & \makecell{$.699$ \\ \scriptsize $.034$}
        & \makecell{$.850$ \\ \scriptsize $.021$}
        & \makecell{$.183$ \\ \scriptsize $.011$}
        % CAMELYON16-PATCH
        & $.660$ & $.330$ & $.643$ & $.772$\\
    \makecell[l]{TransMIL}
        % CAMELYON16
        & \makecell{$.962$ \\ \scriptsize $.009$}
        & \makecell{$.980$ \\ \scriptsize $.004$}
        & \makecell{$.029$ \\ \scriptsize $.014$}
        % NSCLC
        & \makecell{$.950$ \\ \scriptsize $.017$}
        & \makecell{$.970$ \\ \scriptsize $.012$}
        & \makecell{$.046$ \\ \scriptsize $.019$}
        % PANDA
        & \makecell{$.827$ \\ \scriptsize $.074$}
        & \makecell{$.911$ \\ \scriptsize $.030$}
        & \makecell{$.043$ \\ \scriptsize $.021$}
        % BRACS
        & \makecell{$.676$ \\ \scriptsize $.005$}
        & \makecell{$.826$ \\ \scriptsize $.032$}
        & \makecell{$.186$ \\ \scriptsize $.012$}
        % CAMELYON16-PATCH
        &  $.600$ & $.210$ & $.583$ & $.840$ \\
    \makecell[l]{DGR-MIL}
        % CAMELYON16
        & \makecell{$.960$ \\ \scriptsize $.012$}
        & \makecell{$.980$ \\ \scriptsize $.010$}
        & \makecell{$.045$ \\ \scriptsize $.016$}
        % NSCLC
        & \makecell{$.947$ \\ \scriptsize $.024$}
        & \makecell{\underline{$.974$} \\ \scriptsize $.011$}
        & \makecell{$\underline{.038}$ \\ \scriptsize $.022$}
        % PANDA
        & \makecell{$.843$ \\ \scriptsize $.097$}
        & \makecell{$\underline{.933}$ \\ \scriptsize $.047$}
        & \makecell{$.036$ \\ \scriptsize $.025$}
        % BRACS
        & \makecell{$\underline{.703}$ \\ \scriptsize $.033$}
        & \makecell{$.818$ \\ \scriptsize $.035$}
        & \makecell{$.186$ \\ \scriptsize $.023$}
        % CAMELYON16-PATCH
        & $.740$ & $.471$ & $.721$ & $.930$ \\
    \makecell[l]{Bayes-MIL}
        % CAMELYON16
        & \makecell{$.976$ \\ \scriptsize $.007$}
        & \makecell{$.981$ \\ \scriptsize $.006$}
        & \makecell{$\mathbf{.020}$ \\ \scriptsize $.007$}
        % NSCLC
        & \makecell{\underline{$.953$} \\ \scriptsize $.023$}
        & \makecell{$.973$ \\ \scriptsize $.021$}
        & \makecell{$\mathbf{.033}$ \\ \scriptsize $.017$}
        % PANDA
        & \makecell{$.850$ \\ \scriptsize $.060$}
        & \makecell{$.926$ \\ \scriptsize $.031$}
        & \makecell{$.031$ \\ \scriptsize $.016$}
        % BRACS
        & \makecell{$.648$ \\ \scriptsize $.058$}
        & \makecell{$.829$ \\ \scriptsize $.022$}
        & \makecell{$.183$ \\ \scriptsize $.028$}
        % CAMELYON16-PATCH
        & $.793$ & $.551$ & $.772$ & $.862$ \\
    \makecell[l]{AGP}
        % CAMELYON16
        & \makecell{$.883$ \\ \scriptsize $.021$}
        & \makecell{$.954$ \\ \scriptsize $.019$}
        & \makecell{$.069$ \\ \scriptsize $.013$}
        % NSCLC
        & \makecell{$.948$ \\ \scriptsize $.026$}
        & \makecell{$\mathbf{.976}$ \\ \scriptsize $.014$}
        & \makecell{$.048$ \\ \scriptsize $.025$}
        % PANDA
        & \makecell{$.802$ \\ \scriptsize $.086$}
        & \makecell{$.906$ \\ \scriptsize $.047$}
        & \makecell{$\mathbf{.026}$ \\ \scriptsize $.013$}
        % BRACS
        & \makecell{$.634$ \\ \scriptsize $.030$}
        & \makecell{$.830$ \\ \scriptsize $.010$}
        & \makecell{$\mathbf{.134}$ \\ \scriptsize $.014$}   
        % CAMELYON16-PATCH
        & $.842$ & $.340$ & $.826$ & $.953$\\
    \makecell[l]{SGP-MIL}
        % CAMELYON16
        & \makecell{$\mathbf{.980}$ \\ \scriptsize $.007$}
        & \makecell{$\underline{.986}$ \\ \scriptsize $.005$}
        & \makecell{$\underline{.021}$ \\ \scriptsize $.005$}
        % NSCLC
        & \makecell{$\mathbf{.955}$ \\ \scriptsize $.021$}
        & \makecell{$.973$ \\ \scriptsize $.014$}
        & \makecell{$.047$ \\ \scriptsize $.027$}
        % PANDA
        & \makecell{$\mathbf{.900}$ \\ \scriptsize $.065$}
        & \makecell{$\mathbf{.955}$ \\ \scriptsize $.037$}
        & \makecell{$\underline{.028}$ \\ \scriptsize $.022$}
        % BRACS
        & \makecell{$\mathbf{.736}$ \\ \scriptsize $.029$}
        & \makecell{$\mathbf{.870}$ \\ \scriptsize $.026$}
        & \makecell{$\underline{.142}$ \\ \scriptsize $.032$}
        % CAMELYON16-PATCH
        & $\mathbf{.899}$ & $\mathbf{.584}$ & $\mathbf{.877}$ & $\mathbf{.980}$ \\
    \bottomrule
    \end{tabular}
    \caption{Performance on various histopathology datasets. Metrics are mean (top) and standard deviation (bottom). Best performing splits for each model both ACC and AUC-wise were chosen for instance-level evaluation.}
    \label{tab:full_combined_results_no_score}
\end{table*}
