# Supplementary material for: SGPMIL: Sparse Gaussian Process Multiple Instance Learning
Source: arXiv:2507.08711 source file (2026-01-17)
Supplement: Supplementary file 2 [file inducing_points_ablations.tex]

\centering
        \begin{tabular}{lcccccc}
        \toprule
        & \multicolumn{3}{c}{WSI} & \multicolumn{3}{c}{INSTANCE}\\
        \cmidrule(lr){2-4} \cmidrule(lr){5-7}
        \midrule
        $U$ & ACC & AUC & ACE & ACC & AUC & ACE \\
        \midrule
        $16$ & $.971_{.016}$ & $.977_{.020}$ & $.045_{.022}$ & $\underline{.893}$ & $.963$ & $.271$ \\
        
        $32$ & $\underline{.979_{.010}}$ & $\underline{.985_{.005}}$ & $\underline{.026_{.010}}$ & $.880$ & $\underline{.970}$ & $\mathbf{.046}$ \\
        
        $64$ & $.964_{.013}$ & $.981_{.009}$ & $.041_{.016}$ & $.832$ & $.910$ & $.210$\\
        
        $80$ & $\mathbf{.980_{.007}}$ & $\mathbf{.986_{.005}}$ & $\mathbf{.021_{.005}}$ & $\mathbf{.914}$ & $\mathbf{.973}$ & $\underline{.051}$\\
        \bottomrule
        \end{tabular}
    \caption{Performance of SGPMIL on the CAMELYON16 dataset for varying numbers of inducing points ($U$). Slide-level metrics (WSI) and instance-level metrics are reported. Instance-level accuracy (ACC) is computed using the optimal binarization threshold for each model, following the evaluation protocol introduced in BayesMIL.}
    \label{tab:inducing_points_ablations_sgpmil}
