# Supplementary material for: SGPMIL: Sparse Gaussian Process Multiple Instance Learning
Source: arXiv:2507.08711 source file (2026-01-17)
Supplement: Supplementary file 3 [file train_test_times.tex]

\centering
\begin{tabular}{lcc}
\toprule
Model & Training Time (h) & Inference Time (s) \\
\midrule
ABMIL & 5.5 & 0.8 \\
CLAM & 7.0 & 0.9 \\
TransMIL & 13.4 & 1.2 \\
DGRMIL & 16.7 & 1.5 \\
BayesMIL & 9.5 & 1.1 \\
AGP & 31.0 & 6.0 \\
SGPMIL & 9.0 & 1.0 \\
\bottomrule
\end{tabular}
\label{tab:times}
\caption{fjdkl;fasldkfj}
